# Supplementary material for: Federated PCA on Grassmann Manifold for Anomaly Detection in IoT Networks
Source: arXiv:2212.12121 source file (2023-01-10)
Supplement: Supplementary file 1 [file appendix.tex]

%\subsection{Experiment Setting}

\subsubsection{Experimental Evaluation Metrics}
Let $TP, TN, FP$, and $FN$ denote true positive, true negative, false positive, and false negative, respectively. 
\begin{itemize}
	\item Accuracy: $ Acc = \frac{TP + TN}{TP + TN + FP + FN}$.
	%Defined as the percentage of correctly classified records over the total number of records.
	%$$ Acc = \frac{TP + TN}{TP + TN + FP + FN}.$$
	
	\item Precision: $P = \frac{TP}{TP+FP}.$
	%Defined as the \% ratio of the number of True Positive records divided by the sum of True Positives (TP) and False Positive (FP) classified records.
	%$$P = \frac{TP}{TP+FP}.$$ 
	
	\item Recall: $R = \frac{TP}{TP+FN}.$
	%Defined as the \% ratio of number of true positives records divided by the sum of true positives and false negatives (FN) classified records.
	%$$R = \frac{TP}{TP+FN}.$$
	
	\item F1-Score: $ F1 = \frac{2 \times P \times R }{P+R}. $
	%Defined as the harmonic mean of precision and recall and represents a balance between them.
	%$$ F1 = \frac{2 \times P \times R }{P+R}. $$
	
	\item True Positive Rate:
	 $TPR = \frac{TP}{TP + FN}.$
	
	\item False Positive Rate:
	 $FPR = \frac{FP}{FP+TN}. $
	
	%\item \textbf{Receiver Operating Characteristics (ROC)}:
	
\end{itemize}

\comment{
\subsubsection{Dataset}

\begin{table}[htbp!]
	\centering
	\caption{NSL-KDD Dataset}
	\label{tab:tab_appendix}
	\begin{tabular}{|c|c|c|c|c|}
		\hline
		\multirow{2}{*}{\textbf{Category}} & \multicolumn{2}{c|}{\textbf{Training Set}} & \multicolumn{2}{c|}{\textbf{Test Set}}  \\
		\cline{2-5}
		& \#Record & Rate(\%) & \#Record & Rate(\%) \\
		\hline
		\hline
		Normal & 67,343 & 53.46 & 9,711 & 43.08 \\
		\hline
		DoS & 45,927 & 36.46 & 7,458 & 33.08 \\
		\hline
		Probe & 11,656 & 9.25 & 2,421 & 10.74 \\
		\hline
		R2L & 995 & 0.79 & 2,754 & 12.22 \\
		\hline
		U2R & 52 & 0.04 & 200 & 0.89 \\
		\hline
		\hline
		\textit{Total} & \textit{125,973} & \textit{100} & \textit{22,544} & \textit{100} \\
		\hline
	\end{tabular}
\end{table}

NSL-KDD is a popular benchmark networking dataset which has been extensively used for evaluating not only network anomaly detection approaches but also many network security-related tasks. In order to perform our experiments, we use the training set (KDDTrain+) containing 67,343 (53.46\%) benign records and 58,630  (46.54\%) malicious records divided into four attack categories including Denial of Service (DoS), Probing, User-to-Root (U2R), and Remote-to-Local (R2L). For testing purposes, we use the testing set (KDDTest+) comprising 22,544 instances, of which 9,711 (43.08\%) are labeled as normal and 12,833 (56.92\%) are labeled as attack classes. Each record consists of 41 features (3 nominal, 4 binary, and 34 continuous). Table \ref{tab:tab_appendix} shows the statistics of records for the training and test data for normal and different attack classes.
}
%The test data contains 38 traffic classes that include 21 attack classes from the training data, 16 novel attacks, and one normal class.

%Common Attacks \textit{smurf, neptune}. Rare Attacks \textit{satan, ipsweep, portsweep, nmap, back, warezclient, teardrop, pod, guess passwd, buffer overflow, land, warezmaster, imap, rootkit, loadmodule, ftp write, multihop, phf, perl, spy}

\comment{
\begin{table}[t]
	\centering
	\caption{NSL-KDD Dataset}
	\label{tab:tab_3}
	\begin{tabular}{|c|c|c|c|}
		\hline
		\multirow{2}{*}{\textbf{Category}} & \multirow{2}{*}{\textbf{Label}} & \multicolumn{2}{c|}{\textbf{\textit{kddcup.data\_10\_percent.gz}}}  \\
		\cline{3-4}
		&  & \textbf{\# Record} & \textbf{Rate(\%)} \\
		\hline
		\hline
		Normal & normal & 97,278 & 19.6911 \\
		\hline
		\hline
		\multirow{6}{*}{DoS} & back & 2,203 & 0.4459 \\
		%\hline
		& land & 21 & 0.0043 \\
		%\hline
		& neptune & 107,201 & 21.6997 \\
		%\hline
		& pod & 264 & 0.0534 \\
		%\hline
		& smurf & 280,790 & 56.8377 \\
		%\hline
		& teardrop & 979 & 0.1982 \\
		\hline
		%& subtotal & 391,458 & 79.2391 \\
		\hline
		\multirow{4}{*}{Probe} & ipsweep & 1,247 & 0.2524 \\
		%\hline
		& nmap & 231 & 0.0468 \\
		%\hline
		& portsweep & 1,040 & 0.2105 \\
		%\hline
		& satan & 1,589 & 0.3216 \\
		\hline
		%& subtotal & 4,107 & 0.8313 \\
		\hline
		\multirow{8}{*}{R2L} & ftp\_write & 8 & 0.0016 \\
		%\hline
		& guess\_password & 53 & 0.0107 \\
		%\hline
		& imap & 12 & 0.0024 \\
		%\hline
		& multihop & 7 & 0.0014 \\
		%\hline
		& phf & 4 & 0.0008 \\
		%\hline
		& spy & 2 & 0.0004 \\
		%\hline
		& warezclient & 1,020 & 0.2065 \\
		%\hline
		& warezmaster & 20 & 0.0040 \\
		\hline
		%& subtotal & 1,126 & 0.2279 \\
		\hline
		\multirow{4}{*}{U2L} & buffer\_overflow & 30 & 0.0061 \\
		%\hline
		& loadmodule & 9 & 0.0018 \\
		%\hline
		& perl & 3 & 0.0006 \\
		%\hline
		& rootkit & 10 & 0.0020 \\
		\hline
		%& subtotal & 52 & 0.0105 \\
		\hline
		Total &  & 494,021 & 100 \\
		\hline
	\end{tabular}
\end{table}
}
